# Supplementary material for: Learning Robust Representations Of Generative Models Using Set-Based Artificial Fingerprints
Source: arXiv:2206.02067 source file (2022-06-04)
Supplement: Supplementary file 1 [file 00-suppl.tex]

%%%%%%%%%%%%%%%%%%%%%%%%%%%%%%%%%%%%%%%%%%%%%%%%%%%%%%%%%%%%
\appendix
\section{Appendix}

\subsection{Generation of our fake dataset} \label{app:our-dataset-generation}
\paragraph{Effect of using different parameters for data-preprocessing when training generative models}

\begin{figure}[H]
\centering
\begin{subfigure}[b]{0.475\textwidth} 
    \centering
    \includegraphics[width=\textwidth]{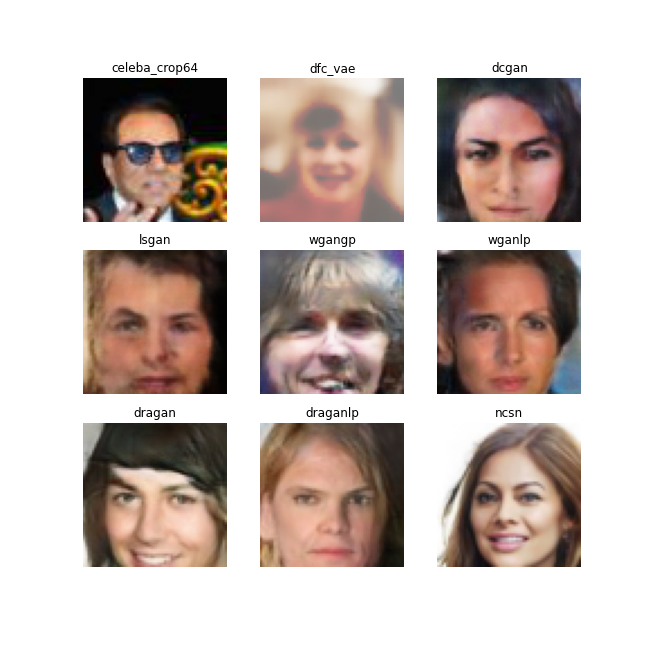}
\end{subfigure}
\hfill
\begin{subfigure}[b]{0.475\textwidth}
    \centering
    \includegraphics[width=\textwidth]{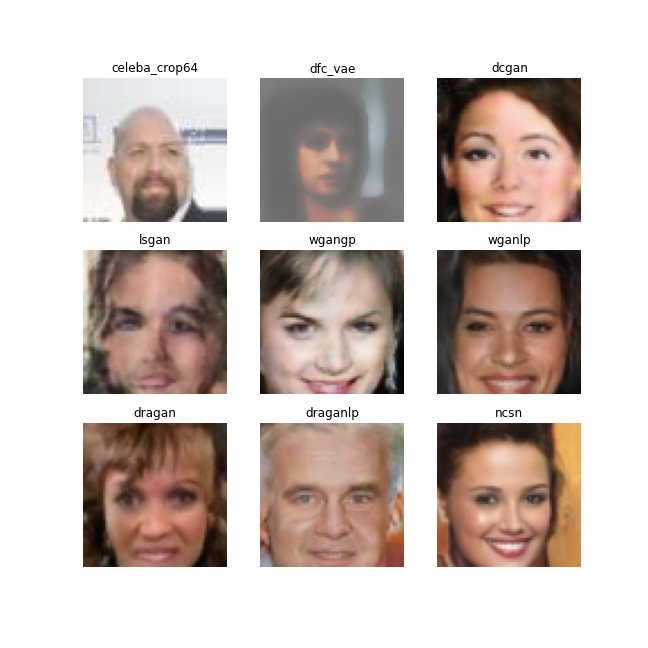}
\end{subfigure}
% new row
\vskip\baselineskip
\begin{subfigure}[b]{0.475\textwidth}
    \centering
    \includegraphics[width=\textwidth]{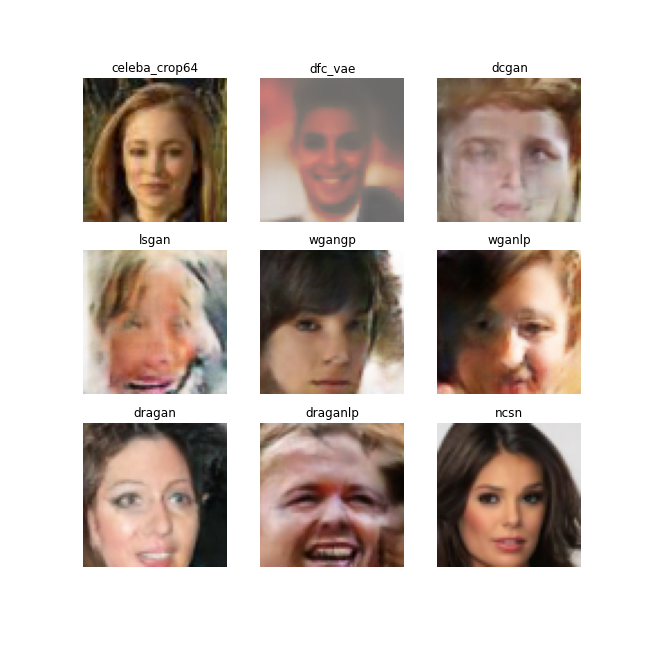}
\end{subfigure}
\hfill
\begin{subfigure}[b]{0.475\textwidth}
    \centering
    \includegraphics[width=\textwidth]{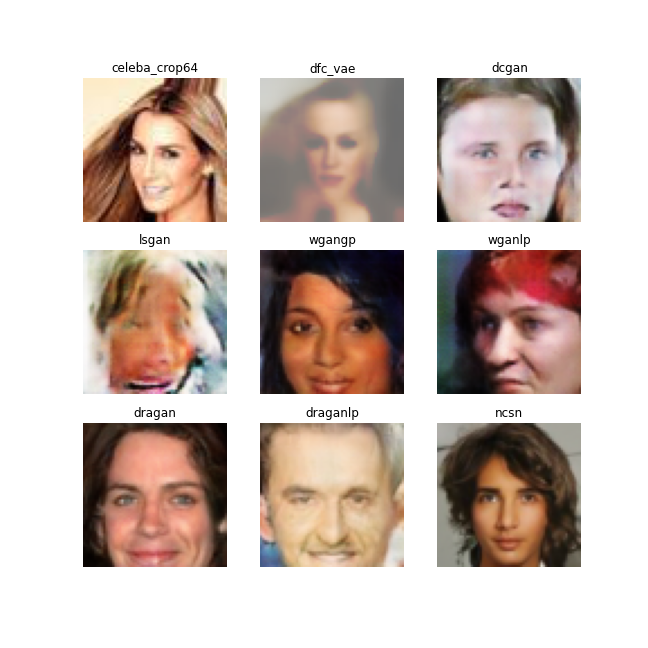}
\end{subfigure}
\caption{Data-preprocessing needs to be consistent to train generative models in our study because our goal is to study the relationship of models and their fingerprints.}
\label{app:images-diff-data-preproc}

\end{figure}

\textbf{Model choices}
- model classes, model names, summary of the architectures
- random initialization: 3 model instances per model setup, each trained on a different initialization (random)

\textbf{Sampling process}
- how we sample from each model class; esp. need details on how to sample from the score-based models

\textbf{Training process}
- how we train each model: we use the same dataset, with consistent preprocessing to train all models. This protocol allows us to study the effect of model variations on their fingerprints, separately from any potential effects from the choice of datasets and tasks enforced to train the models.

\subsection{Fingerprints of Generative Models} \label{app:our-model-fingerprints}
Here we show fingerprints of four generative models that represents each model class.
VAE: 
Flow:
GAN:
Score-based:
\subsection{Implementation Details} \label{app:implementation-details}
\paragraph{Our Set-Encoder} \label{app:our-set-encoder}

\paragraph{Source Attribution: Classifier} \label{app:model-src-classifier}

\subsection{Bound of Decorrelation Score} \label{app:decorrel-score-bound}
%todo

\subsection{Ablation}
\begin{table}[t]
    \centering
    \begin{tabular}{cccccccccc}
    \hline
        n\_bags per model & Block Correl. Score & AUC (\%)  \\ \hline \hline
        1 & $0.581\pm 0.032$ & $55.3 \pm 1.334$  \\ \hline
        5 & $0.678 \pm  0.023$ & $64.4 \pm  1.251$  \\ \hline
        10 & $0.682 \pm  0.019$ & $63.1 \pm  1.023 $ \\ \hline
        25 & $0.703 \pm  0.018$ & $64.7 \pm  1.022 $ \\ \hline
        50 & $0.782 \pm  0.017$ & $72.4 \pm  1.013$  \\ \hline
        100 & \textbf{$0.838 \pm  0.013$} & \textbf{$76.9 \pm  0.873$}  \\ \hline
        200 & $0.822 \pm  0.011 $ & $77.3 \pm  0.822 $ \\ \hline
        300 & $0.818 \pm  0.009 $ & $78.9 \pm  0.723 $ \\ \hline
    \end{tabular}
\end{table}
